# Supplementary material for: Synthetic Combinations: A Causal Inference Framework for Combinatorial Interventions
Source: arXiv:2303.14226 source file (2024-01-15)
Supplement: Supplementary file 1 [file natural_model.tex]

\section{Natural Model Satisfying Assumption \ref{ass:donor_set_identification}}
\label{sec:natural_model}
In this section, we describe a simple model such that the properties of Assumption \ref{ass:donor_set_identification} hold. 
For every unit $n$, suppose  $\balpha_n \in \{\balpha(1) = (1,1,1,0\ldots,0), \balpha(2) =(1,1,2,0\ldots,0),\balpha(3) = (1/8,1/8,1/8,0\ldots,0), \balpha(4) = (1/8,1/8,1/4,0\ldots,0)\}$.
It is easy to verify that $\text{rank}(\mathcal{A}) = 2 $.
Next, we define the observation pattern to be such that the potential outcome $\E[Y_n^{(\pi)}]$ for a unit-combination pair $(n,\pi)$ is only observed if $| \langle \balpha_n, \bchi^{\pi} \rangle | \geq 1$. 
That is, $Y_{n\pi} = \star$ if $  | \langle \balpha_n, \bchi^{\pi} \rangle | < 1$, and $Y_{n\pi} = \E[Y_n^{(\pi)}]$ if otherwise. 
This treatment assignment induces unobserved confounding since the treatment assignment $\mathcal{D}$ is a function of the Fourier coefficients $\mathcal{A}$. 
This missingness pattern where outcomes with larger absolute values are observed is common in applications such as recommendation engines, where we are only likely to observe ratings for combinations that users either strongly like or dislike.
Next, observe that $| \langle \balpha(3), \bchi^{\pi} \rangle | \leq 3/8$ and $| \langle \balpha(4), \bchi^{\pi} \rangle | \leq 1/2$ for all combinations $\pi \in \Pi$. 
Hence, we observe \emph{zero} outcomes for units with Fourier coefficient type belonging to $\{\balpha(3),\balpha(4)\}$.
For units with type belonging to $\{\balpha(1),\balpha(2)\}$, we observe at least the combinations $\{\pi_1, \pi_2,\pi_3\}$ with associated Fourier characteristics: $\{\bchi^{\pi_1} = (1,1,1,1,\ldots,1), \bchi^{\pi_2} = (-1,1,1,1,\ldots,1), \bchi^{\pi_3} = (1,-1,1,1,\ldots,1)$. 
One can check that these observed combinations ensure that horizontal span inclusion holds for  for units with type $\{\balpha(1),\balpha(2)\}$.
Further, since $\text{rank}\{\balpha(1),\balpha(2)\} =2$, vertical span inclusion also holds.
