# Supplementary material for: Synthetic Combinations: A Causal Inference Framework for Combinatorial Interventions
Source: arXiv:2303.14226 source file (2024-01-15)
Supplement: Supplementary file 3 [file lasso_proofs.tex]

\section{Lasso Horizontal Regression Analysis}
\label{sec:Lasso_finite_sample_analysis}

\begin{proposition} 
\label{prop:Lasso_convergence_rate} 
Let Assumptions \ref{ass:observation_model}, \ref{ass:subgaussian_noise}, and \ref{ass:incoherence} hold. Then, conditioned on $\mathcal{A}$, we have
\begin{equation}
\label{eq:Lasso_convergence_rate}
 \hat{\E}[Y_u^{(\pi)}] - \E[Y_u^{(\pi)}] = O_p\left(\sqrt{\frac{s^2p}{|\Pi_u|}} ~ \bigg | ~ \mathcal{A} \right) 
\end{equation}
for any donor unit $u \in\mathcal{I}$ and $\pi \in \Pi$
\end{proposition}

\begin{proof} We have
\begin{align*}
     \hat{\E}[Y_u^{(\pi)}] - \E[Y_{u}^{(\pi)}] & = \langle  \hat{\balpha}^L_u, \bchi^{\pi} \rangle - \langle  \balpha_u, \bchi^{\pi} \rangle \\
     & = \langle  \hat{\balpha}^L_u - \balpha_u, \bchi_{\pi} \rangle \\
     & \leq \lVert \hat{\balpha}^L_u - \balpha_u \rVert_1 \lVert \bchi_{\pi} \rVert_{\infty}\\ 
     & = \lVert \hat{\balpha}^L_u - \balpha_u \rVert_1
\end{align*}
Then, using the result of Theorem 2.18 in  \cite{rigollet2015high} yields the claimed result. 
\end{proof}
